# Supplementary material for: A new look at the infrared properties of z $\sim$ 5 galaxies
Source: arXiv:2210.09312 source file (2022-10-17)
Supplement: Supplementary file 1 [file hyperlink_hack.tex]

%-----------------------------------------
% avoids the 
%   \pdfendlink ended up in different nesting level than \pdfstartlink.\AtBegShi@Output ...ipout \box \AtBeginShipoutBox
% error
%-----------------------------------------
%
% see https://tex.stackexchange.com/questions/249579/pdfendlink-ended-up-in-different-nesting-level-than-pdfstartlink-error-with

% different workaround
%\AtBeginShipout{%
%  \ifnum\value{page}>1 %
%    \typeout{* Additional boxing of page `\thepage'}%
%    \setbox\AtBeginShipoutBox=\hbox{\copy\AtBeginShipoutBox}%
%  \fi
%}

\usepackage{etoolbox}
\makeatletter
\newcount\c@additionalboxlevel
\setcounter{additionalboxlevel}{0}
\newcount\c@maxboxlevel
\setcounter{maxboxlevel}{1}
\patchcmd\@combinedblfloats{\box\@outputbox}{%
  \stepcounter{additionalboxlevel}%
  \box\@outputbox
}{}{\errmessage{\noexpand\@combinedblfloats could not be patched}}

\AtBeginShipout{%
  \ifnum\value{additionalboxlevel}>\value{maxboxlevel}%
    \typeout{Warning: maxboxlevel might be too small, increase to %
      \the\value{additionalboxlevel}%
    }%
  \fi 
  \@whilenum\value{additionalboxlevel}<\value{maxboxlevel}\do{%
    \typeout{* Additional boxing of page `\thepage'}%
    \setbox\AtBeginShipoutBox=\hbox{\copy\AtBeginShipoutBox}%
    \stepcounter{additionalboxlevel}%
  }%
  \setcounter{additionalboxlevel}{0}%
}
\makeatother
