# Supplementary material for: A new look at the infrared properties of z $\sim$ 5 galaxies
Source: arXiv:2210.09312 source file (2022-10-17)
Supplement: Supplementary file 4 [file journals.tex]

% Astrophysics and Space Science
              % Planetary and Space Science
