# Supplementary material for: A new look at the infrared properties of z $\sim$ 5 galaxies
Source: arXiv:2210.09312 source file (2022-10-17)
Supplement: Supplementary file 5 [file package.tex]

\usepackage{txfonts}
\usepackage[T1]{fontenc}
\usepackage{ae,aecompl}

\usepackage{graphicx}

% to avoid conflict let amsmath redefine some stuff
\let\iiint=\relax
\let\iiiint=\relax
\let\idotsint=\relax
\let\iint=\relax
\usepackage{amsmath}
\usepackage{amsfonts}
\usepackage{amssymb}

\usepackage{xcolor}

\usepackage{breakcites}
\usepackage{hyperref}
\usepackage{footnote}

\usepackage{comment}

\usepackage{xfrac}
